# Supplementary material for: UnMask: Adversarial Detection and Defense Through Robust Feature Alignment
Source: arXiv:2002.09576 source file (2020-11-14)
Supplement: Supplementary file 1 [file 06-appendix.tex]

\section*{Appendix}\label{appendix}

In the supplemental appendix we provide additional information on the experimental setup in Section~\ref{detailed_setup}; 
selection of the adversarial training parameter, $\epsilon$, in Section~\ref{sec:line-search};
conversion of the PASCAL-Part dataset for use in the \dataset{} in Section~\ref{extra_dataset_info};
and information on how to setup and run the open-sourced code and models presented in this paper in Section~\ref{code_and_models}.

\section{Detailed Experiment Setup}\label{detailed_setup}
All experiments were tested in a Linux environment using Python 3, on 2 Nvidia Titan X GPUs, a Titan RTX and an Nvidia DGX. We note that a single Nvidia GPU is sufficient to recreate all of the experiments, however, we recommend that the GPU has at least 12GB of memory (not tested with less).
Anaconda 3 is used to manage all the Python packages. To facilitate reproducibility of the Python environment, we release an Anaconda YAML specification file of the libraries utilized in the experiments. This allows the user to create a new virtual Python environment with all of the packages required to run the code by importing the YAML file.
In addition, we use multiple Github repositories in the code base---(i) for the Mask R-CNN model \cite{matterport} and (ii) to assist in the development of the \dataset{}
\footnote{We utilized part of the following repositories to convert the PASCAL-Part dataset to Microsoft COCO format: \href{https://github.com/waspinator/pycococreator}{I}}. Since there are significant modifications from the original implementation, it's necessary for the user to utilize the provided version.

\section{Adversarial Training: Finding Train Epsilon}\label{sec:line-search}
We follow standard procedure and determine the optimal $\epsilon$ on a per-dataset basis (class set in our case)~\cite{madry2017towards}, conducting a line search across $\epsilon$=\{1, 2, 4, 6, 8, 16\}.
We select the $\epsilon$ with best generalization performance on the validation set, for each class set (e.g., cs3a, cs5b). 
We find that $\epsilon$=4, provides the best performance across each class sets, as seen in Figure~\ref{fig:line_search}. While $\epsilon$=6 appears to be a good choice for class set CS3a, it has poor generalization performance and overfits to PGD-$L_\infty$. This can be seen through the bar chart of Figure~\ref{fig:line_search-detailed}, where selecting an $\epsilon$ greater than 4 reduces the generalization of adversarial training to all other attack vectors. For this reason, we select $\epsilon$=4 for all class sets.

\begin{figure}[tb]
\centering
\includegraphics[width=0.9\linewidth]{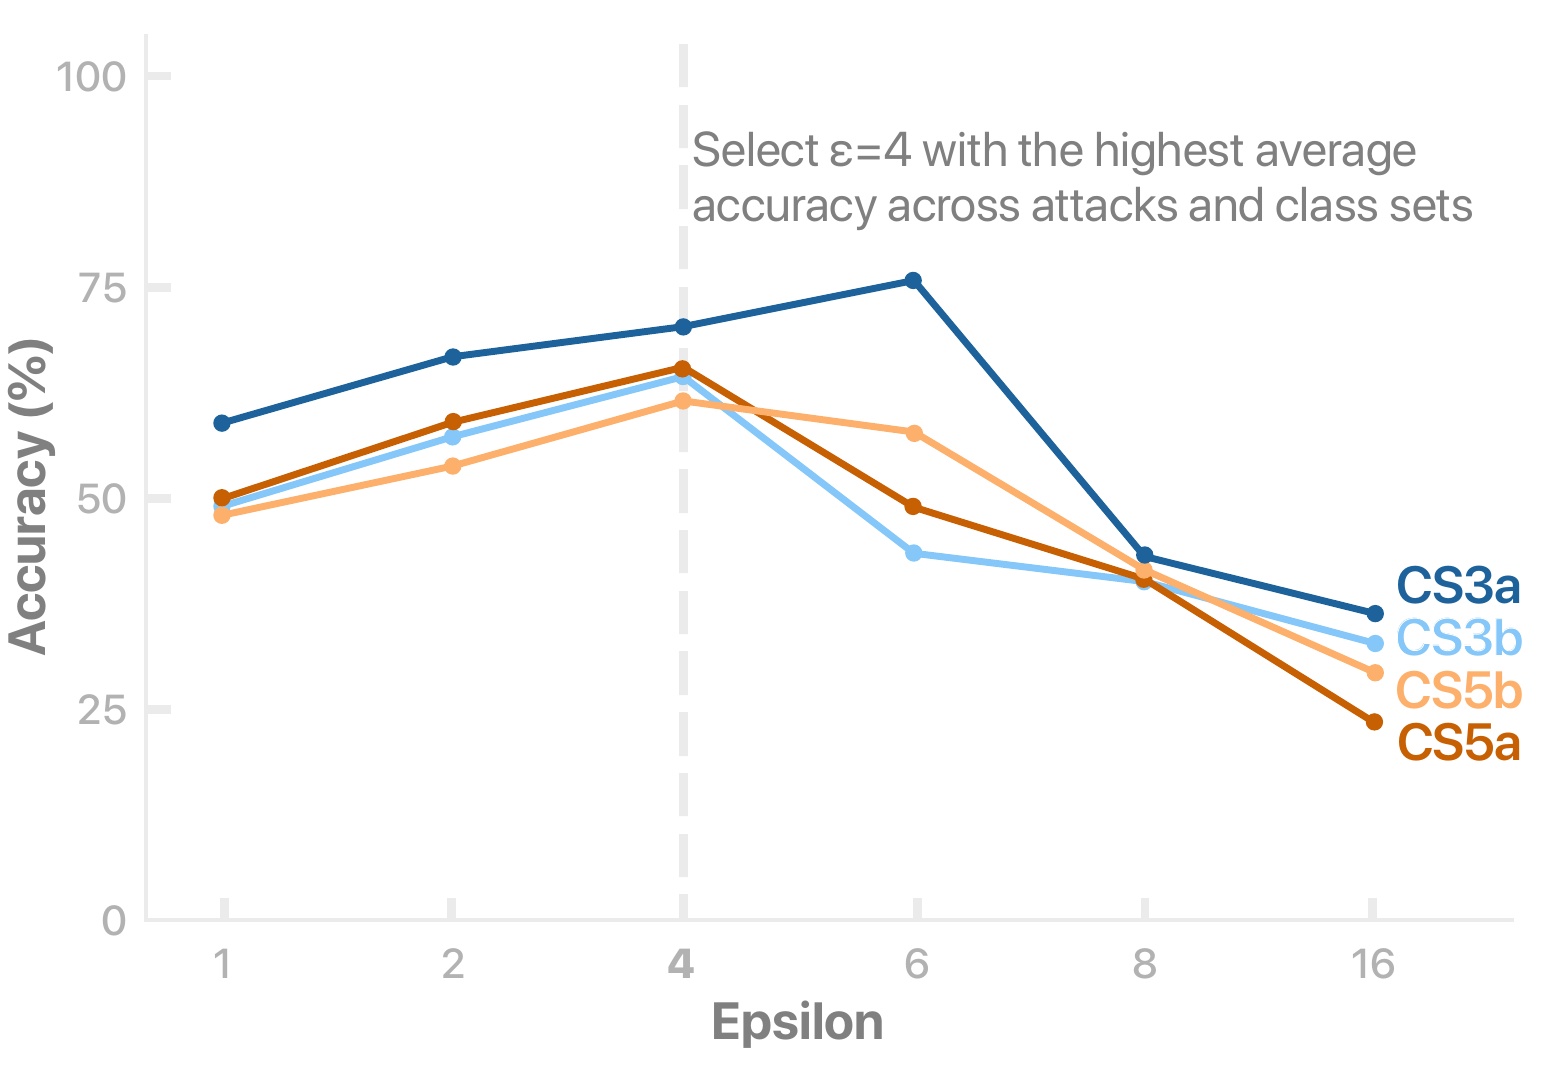}
\caption{Line search for adversarial training parameter $\epsilon$ on validation data. We select $\epsilon$=4, since it provides the best performance on most attacks.
}
\label{fig:line_search}
\end{figure}

\begin{figure}[tb]
\centering
\includegraphics[width=\linewidth]{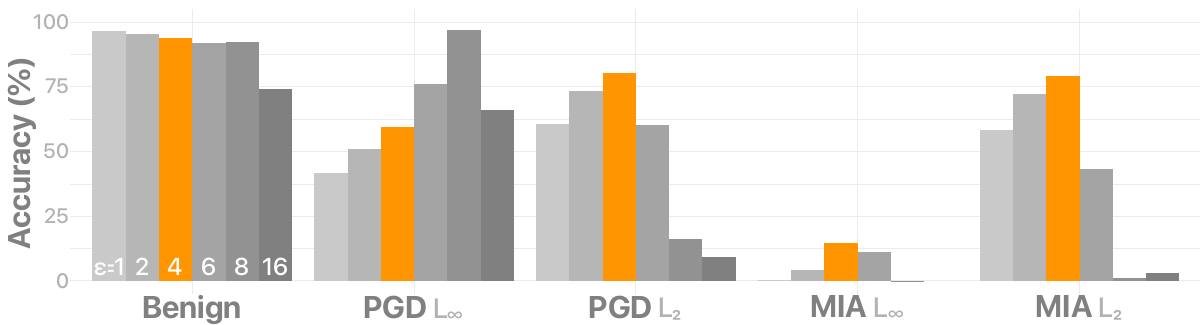}
\caption{Detailed bar chart describing the performance of $\epsilon$ across all attack vectors. We select $\epsilon$=4, since it provides the best performance on most attacks.
}
\label{fig:line_search-detailed}
\end{figure}

\section{Extended \dataset{} Information}\label{extra_dataset_info}
In Table~\ref{feature_matrix}, the class-feature matrix describes the features contained by each class in the dataset.
In Table \ref{feature_mapping}, we can see that the features in the \dataset{} are a generalization of the ones in PASCAL-Part. For example, the PASCAL-Part dataset has 18 variations of the leg feature, however, in order to create a model that better generalizes, we combine this to a single leg feature. We note that in Table \ref{feature_matrix}, that two features have multiple sub-features condensed into a single feature (not listed due to space constraints). 
These features are: vehicle: \{vehicle left, vehicle right, vehicle top, vehicle back\} and coach: \{coach left, coach right, coach back, coach top, coach front\}.
In addition, we note that there is a minor error in the conversion of the handlebar feature in the bike and motorcycle class (handlebar features were labeled as hand). However, since those classes are not utilized in the experiments, the effects are minimized.

\section{Code and Models}\label{code_and_models}
We open-source all of the code, data and models used in this paper. Below, we provide a walk-through of how to set up the environment and run the code locally. For additional information, and the steps necessary to train a custom feature extraction model $K$, we provide a detailed walk through on Github (\url{https://github.com/unmaskd/unmask}).

\textbf{Setup.} Below are the steps the user should take in order to set up their environment for running the code:

\begin{enumerate}
    \item Set up a Linux environment (not tested for Windows) with an Nvidia GPU containing at least 12GB of memory (less may work, but not tested).
    \item Download the open-sourced code, dataset and models from Github.
    \item Create a virtual Python environment using the provided YAML configuration file on Github.
    \item Activate the new virtual Python environment
\end{enumerate}

\textbf{Running the code.} Once the environment is set up, we can control the experiment parameters from the config.py file and run the code in main.py.
